# Supplementary material for: Improved Spin-State Energy Differences of Fe(II) molecular and crystalline complexes via the Hubbard U-corrected Density
Source: arXiv:2101.07035 source file (2021-01-18)
Supplement: Supplementary file 1 [file SI.pdf]

# Supporting information for: Improved Spin-State Energy Differences of Fe(II) molecular and crystalline complexed *via* the Hubbard $U$-corrected Density

Lorenzo A. Mariano,[†] Bess Vlaisavljevich,[‡] and Roberta Poloni[*,†]

†*Grenoble-INP, SIMaP, University of Grenoble-Alpes, CNRS, F-38042 Grenoble, France*

‡*University of South Dakota, Vermillion, South Dakota, 57069 USA*

E-mail: roberta.poloni@grenoble-inp.fr

# DFT calculations

All calculations (DFT, CCSD(T) and CASPT2) on the six Fe(II) complexes $[Fe(H_2O)_6]^{+2}$, $[Fe(NH_3)_6]^{+2}$, $[Fe(NCH)_6]^{+2}$, $[Fe(PH_3)_6]^{+2}$, $[Fe(CNH)_6]^{+2}$ and $[Fe(CO)_6]^{+2}$ are computed using the TPSSh-optimized geometries reported in Ref. S1. The PBE, PBE+U and PBE+U+V $\Delta E_{\text{H-L}}$ calculations are performed by using Quantum ESPRESSO.[S2,S3] We use the GBRV ultrasoft pseudopotentials[S4,S5] with wavefunction and charge density cutoffs of 80 Ry and 800 Ry, respectively. The Makov-Payne correction[S6] is added to the total energy calculations of isolated charged systems. The other DFT single point energy calculations are performed using ORCA[S7] with a tight integration grid (grid6) and aug-cc-pVTZ basis sets. For the density analysis, we use PAW pseudopotentials[S8] from the PSlibrary[S9] to compute the all-electron charge density. In this case we use 130 Ry and 900 Ry for the wavefunction and charge density cutoff respectively. $U_{\text{sc}}$ and $V_{\text{sc}}$ are recomputed in this case (see Tabs. S2 and S3). The calculations of the five molecular crystals $Fe(phen)_2(NCS)_2$, $Fe(abpt)_2(NCS)_2$, $Fe(abpt)_2(NCSe)_2$, $Fe[HB(pz)_3]_2$ and $FeL_2[BF_4]_2$, are performed using Quantum ESPRESSO. The geometrical optimization is performed using the .cif files available on the Cambridge Structural Database. The PBE functional together with the semiempirical Grimme's D3 van der Waals correction[S10] combined with the Becke-Johnson (BJ) damping scheme[S11] is used. The Hubbard $U_{\text{sc}}$ is then computed once on the optimized geometry (i.e. without computing a structurally consistent $U$). The same wavefunction and charge density cutoffs used for the six small molecules are employed. A $2\times2\times2$ Monkhorst-Pack grid is used for both geometrical optimization and the Hubbard $U$ calcsulations. Because for these crystals we compare with $\Delta E_{\text{H-L}}$ values computed using TPSSH and M06L by Vela and coworkers obtained on isolated molecules, we also extract the molecular version of these crystals from the periodic calculations. These structures are used to compute PBE[U] and PBE[HF] for the gas phase calculations of the molecular crystals. For $[Fe(tacn)_2]^{+2}$ and $[Fe(bpy)_3]^{+2}$ we optimize the structure using TPSSh with ORCA. For the seven molecular complexes we compute PBE[HF], TPSSh, and M06-L single point energies with a aug-cc-pVTZ basis set

for Fe and cc-pVTZ for the other atoms together with a tight integration grid. For all these calculations we add the D3 correction with the BJ damping scheme, except for M06-L for which this is not implemented. In this case we use D3 without the BJ damping. The PBE[U] calculations of $[Fe(tacn)_2]^{+2}$ and $[Fe(bpy)_3]^{+2}$ and the five gas phase version of the molecular crystals are instead performed using Quantum ESPRESSO, using large unit cells to avoid interaction between images.

# CASPT2

The computational procedure adopted here is similar to Ref. S1. The CASPT2 calculations are peformed using the extended-multistate approach (XMS) with a real vertical shift of 0.2 a.u.and a Cholesky decomposition of the two-electron integrals. The three lowest states were state-avaraged and treated with XMS-CASPT2 for HS while only one state was computed for LS. Scalar relativistic effects were included using a second-order Douglas-Kroll-Hess (DKH) Hamiltonian while spin-orbit coupling was not considered.[S12]

By adopting the TPSSh geometries without any symmetry constraint, we were unable to converge a (10e,12o) active space for $[Fe(H_2O)_6]^{2+}$ in LS where the two ligand $e_g$ orbitals remained in the active space after orbital optimization. The Fe 3s orbital consistently rotated into the active space replacing one of the $e_g$ orbitals. This implies that for this particular molecule using the smaller active space should not impact the HS-LS energy splitting significantly, as discussed in more detail in the SI of Ref. S1. For this reason, the CASPT2 calculations used for the CASPT2/CC reference for water are performed using the (6e,10o) active space.

The extrapolation to the complete basis set (CBS) limit was performed by fitting three energy values computed using the cc-pVTZ-DK, cc-pVQZ-DK, and cc-pV5Z-DK basis sets. The CASSCF and the CASPT2 energies were fitted separately by adopting the procedure by Feller[S13,S14] and Helgaker et al.,[S15] respectively. The CASSCF energy is extrapolated us-

ing the $a+b\exp(-cX)$ function while for the second-order energy correction we use $a+bX^{-3}$. The $\Delta E_{\text{H-L}}$ computed using CASPT2 and the cc-pVTZ-DK, cc-pVQZ-DK, and cc-pV5Z-DK basis sets, respectively, are reported in Tab. S1. All the calculations are performed without any empirical correction applied to the zeroth-order Hamiltonian used for CASPT2, i.e. the so-called ionisation potential-electron affinity (IPEA) shift. In the SI of our previous study we have reported a comparison between calculations performed without and with an IPEA shift of 0.25 a.u. The $\Delta E_{\text{H-L}}$ always decrease upon inclusion of the IPEA shift and the largest deviation was found to be 173 meV for NCH.[S1]

Table S1: CASPT2 values of $\Delta E_{\text{H-L}}$ in eV for computed using the three basis sets. The last column shows the final energies obtained upon extrapolation (performed separately for CASSCF and CASPT2) to the limit of complete basis set.

| $\Delta E_{\text{H-L}}$ / **CASPT2** | | | | |
|---|---|---|---|---|
| Complex | Basis Set | | | |
| | cc-pVTZ-DK/DKH | cc-pVQZ-DK/DKH | cc-pV5Z-DK/DKH | CBS |
| $H_2O$ | -2.161 | -2.064 | -2.021 | -1.990 |
| $NH_3$ | -1.053 | -0.942 | -0.896 | -0.846 |
| NCH | -0.518 | -0.382 | -0.323 | -0.265 |
| $PH_3$ | 1.642 | 1.982 | 2.154 | 2.308 |
| CO | 1.505 | 1.650 | 1.717 | 1.783 |
| CNH | 2.355 | 2.524 | 2.595 | 2.661 |

# CCSD(T)

The 3s3p correlation contribution computed using CCSD(T) to yield the final CASPT2/CC results are taken from our previous work.[S1] We therefore refer the reader to the SI of that work for a detailed discussion.

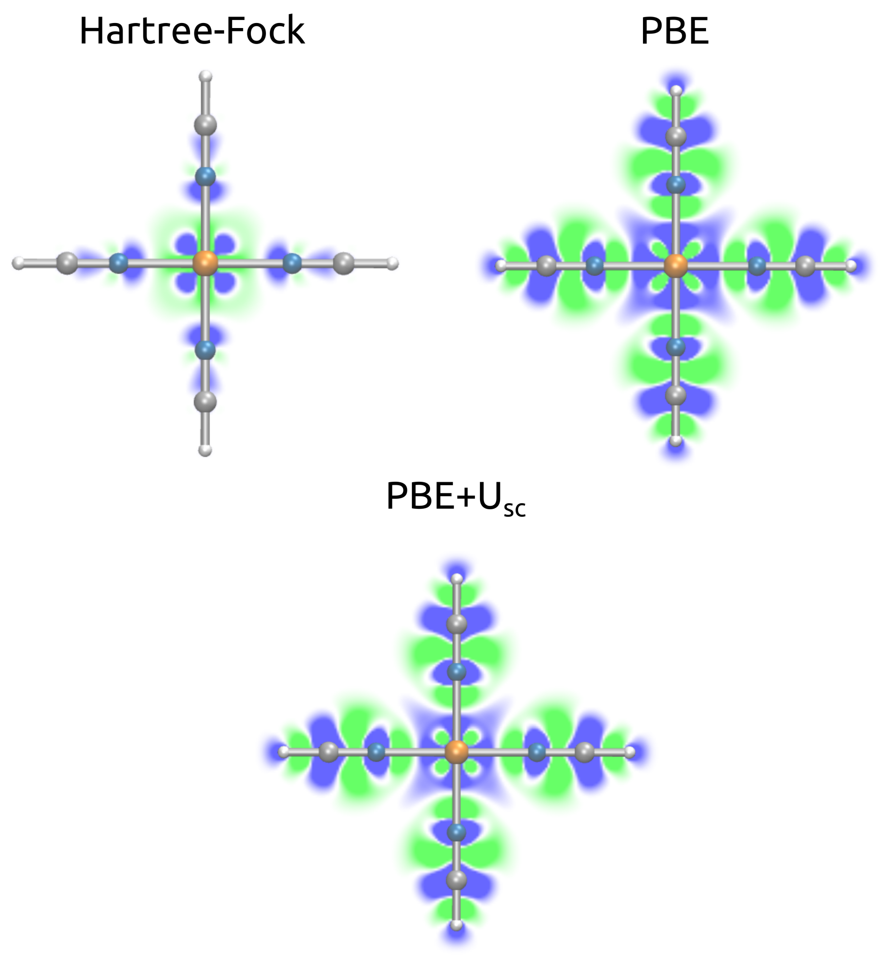


Figure S1: Density difference plot, $\delta\rho_{\mathrm{x}}(r)$ (see text), for $[\mathrm{Fe(NCH)_6}]^{+2}$ between x=[PBE, PBE+U, HF] and the relaxed CASPT2 density; green and blue correspond to positive and negatives values, respectively. The plot shows values between -0.005 $e/\mathrm{bohr}^3$ and 0.005 $e/\mathrm{bohr}^3$.

## Projectors in DFT+U

Within the DFT+U approach the energy is written as:

$$E_{\text{DFT+U}}[\rho(\mathbf{r}), \{n_m^\sigma\}] = E_{\text{DFT}}[\rho(\mathbf{r})] + \sum_{m,\sigma} \frac{U}{2}[n_m^\sigma(1 - n_m^\sigma)] \quad (1)$$

where $\{|\phi_m\rangle\}$ are the chosen atomic-like functions and the occupations, $\{n_m^\sigma\}$, are the eigenvalues of the 5×5 occupation matrix $n_{mm'}^\sigma = \sum_i f_i^\sigma \langle\Psi_i^\sigma|\phi_m\rangle \langle\phi_{m'}|\Psi_i^\sigma\rangle$, with $f_i^\sigma$ being Fermi-Dirac occupations. In Quantum ESPRESSO it is possible to choose among atomic orbitals obtained by solving the Schrödinger equation for the isolated atom, as they are or, alternatively, by applying an orthogonalisation procedure based on Löwdin decomposition in order to obtain a localised basis set with zero overlap with the neighbour atomic basis (ortho-atomic projectors). We find a significant difference in the values of $U$ and, consequently, in the computed $\Delta E_{\text{H-L}}$ when the atomic and ortho-atomic projects are used (see Tab. S2). The $\Delta E_{\text{H-L}}$ reported in the manuscript are computed using the so called ortho-atomic projectors while in our previous work[S1] we employed the atomic ones.

Table S2: $U_{\text{sc}}$ and $\Delta E_{\text{H-L}}$ (in eV) computed using ortho-atomic and atomic projectors. In parentheses the values computed using PAW pseudopotentials to extract the all-electrons charge density (see text).

| Complex | ortho-atomic | | | atomic | | |
|---|---|---|---|---|---|---|
| | Hubbard $U_{\text{sc}}$ | | $\Delta E_{\text{H-L}}$ | Hubbard $U_{\text{sc}}$ | | $\Delta E_{\text{H-L}}$ |
| | LS | HS | | LS | HS | |
| $[Fe(H_2O)_6]^{+2}$ | 9.58 | 9.10 | -1.50 | 7.02 | 6.45 | -1.33 |
| $[Fe(NH_3)_6]^{+2}$ | 9.10 (6.81) | 8.22 | -0.44 | 7.30 | 6.23 | -0.22 |
| $[Fe(NCH)_6]^{+2}$ | 9.45 (7.84) | 9.13 | 0.21 | 8.54 | 6.82 | 0.56 |
| $[Fe(PH_3)_6]^{+2}$ | 8.97 | 7.19 | 1.81 | 9.39 | 6.22 | 2.17 |
| $[Fe(CO)_6]^{+2}$ | 9.43 (8.61) | 8.06 | 2.64 | 9.89 | 6.61 | 3.08 |
| $[Fe(CNH)_6]^{+2}$ | 9.47 (8.71) | 8.26 | 3.23 | 10.07 | 6.84 | 3.65 |
| $Fe(phen)_2(NCS)_2$ | 9.61 | 7.62 | -0.07 | 9.22 | 6.65 | 0.24 |
| $Fe(abpt)_2(NCS)_2$ | 9.48 | 7.40 | 0.09 | 8.94 | 6.64 | 0.47 |
| $Fe(abpt)_2(NCSe)_2$ | 9.42 | 6.83 | 0.16 | 8.88 | 6.17 | 0.45 |
| $Fe[HB(pz)_3]_2$ | 9.31 | 6.72 | 0.18 | 8.71 | 5.38 | 0.52 |
| $FeL_2[BF_4]_2$ | 9.48 | 7.90 | 0.20 | 9.07 | 6.66 | 0.52 |
| $[Fe(tacn)_2]^{+2}$ | 8.92 | 7.69 | | | | |
| $[Fe(bpy)_3]^{+2}$ | 9.30 | 8.25 | | | | |

# Linear-response $U$ and $V$

DFT+U$_{sc}$ and DFT+U$_{sc}$+V$_{sc}$ calculations are performed using linear-response to evaluate the Hubbard parameters $U$ and $V$.[S16–S18] The Hubbard V$_{IJ}$ parameter between atomic sites I and J is computed from the interacting and non-interacting response functions $\chi_{IJ}$ and $\chi^0_{IJ}$ as:

$$V_{IJ} = (\chi_0^{-1} - \chi^{-1})_{IJ}, \tag{2}$$

and the on-site $U$ parameter of DFT+U is the special case V$_{II}$. Within the DFT+U$_{sc}$ calculations we evaluate the $U$ on the iron with an home-made script by computing the response functions $\chi = \partial n/\partial\alpha$ and $\chi^0 = \partial n^0/\partial\alpha$ from a linear regression between the relative change of the screened (self-consistent) and bare occupations, i.e $n$ and $n^0$, respectively, and the applied perturbation $\alpha$, as explained in Ref. S16. This is done iteratively. Because the ground state changes upon inclusion of the Hubbard correction, the $U$ computed on the DFT ground state may be different than the one computed on the DFT+U one.[S19] Thus a self-consistent linear-response $U$ calculation is implemented where a first linear-response calculation is performed on the U=0 ground-state, and then the computed $U$ is used to obtained a new DFT+U ground-state density upon which a further linear-response $U$ calculation is run. This is repeated until the $U$ used to obtain the unperturbed charge density is close to the output linear-response $U$. We impose a convergence threashold of 0.05 eV between input and output $U$ which is usually achieved in 2-3 steps.

The DFT+U+V calculations were performed by adopting the approach reported in Ref. S18 based on the density-functional perturbation theory to computed the on-site V$_{II}$ (i.e. $U$) and the inte-site V$_{IJ}$ between the iron site, $I$, and the six first neighbouring atoms, $J$, as implemented in the *hp.x* utility of Quantum ESPRESSO. Because of the Jahn-Teller distortion at the high spin state, the computed inter-site V$_{IJ}$ adopt three different values corresponding to the three M-L lengths. The computed Hubbard parameters used for the DFT+U$_{sc}$ and DFT+U$_{sc}$+V$_{sc}$ calculations are reported in Tab. S2 and S3.

Table S3: $U_{\mathrm{sc}}$ and $V_{\mathrm{sc}}$ (in eV) used for the DFT+U+V calculations computed using the density-functional perturbation theory as reported in Ref. S18 using the *hp.x* routine. In parentheses the values computed using the PAW pseudopotentials to extract the all-electron charge density.

| Complex | on-site $U_{sc}$ | | inter-site $V_{sc}$ | |
|---|---|---|---|---|
| | Low Spin | High Spin | Low Spin | High Spin |
| $[Fe(H_2O)_6]^{+2}$ | 9.00 | 10.58 | 0.54 | 0.47, 0.36, 0.33 |
| $[Fe(NH_3)_6]^{+2}$ | 8.68 (6.55) | 9.54 | 0.36 (0.61) | 0.07, 0.06, 0.04 |
| $[Fe(NCH)_6]^{+2}$ | 9.84 (8.02) | 11.54 | 1.42 (1.54) | 1.23, 1.15, 1.07 |
| $[Fe(PH_3)_6]^{+2}$ | | | | |
| $[Fe(CO)_6]^{+2}$ | 9.26 (9.27) | 10.13 | 1.05 (1.17) | 0.98, 0.94, 0.75 |
| $[Fe(CNH)_6]^{+2}$ | 9.41 (8.34) | 10.01 | 1.14 (1.15) | 1.07, 1.06, 0.93 |

# Effect of the geometry on the $\Delta E_{\textbf{H-L}}$

Tabs. S4 and S5 report the adiabatic energy differences, $\Delta E_{\text{H-L}}$, computed for $[Fe(NH_3)_6]^{+2}$ and $[Fe(CO)_6]^{+2}$ using 11 different functionals. For each functional we use five geometries (PBE+U, PBE, TPSSh, B3LYP and PBE0). For HS, the Jahn-Teller distorsion yields non-identical metal-ligand (M-L) bond lengths. Tab. S6 reports the (averaged) M-L distances for (HS) LS at different geometries. For this specific study, the PBE[U] calculations are performed using atomic projectors because the ortho-atomic ones yiels a slower convergence in the case of HS. For each geometry, we compute the corresponding $U_{\text{sc}}$ (see Tab. S7). The PBE+U geometries are computed using a structurally consistent $U$ and are taken from our previous work.[S1]

Table S4: $\Delta E_{\text{H-L}}$ (eV) of $Fe(NH_3)_6]^{2+}$ computed with different functionals using five geometries (PBE+U, PBE, TPSSh, B3LYP, PBE0).

| | $\Delta E_{\text{H-L}}$ | | | | |
|---|---|---|---|---|---|
| Geometry → Functional ↓ | PBE+U | PBE | TPSSh | B3LYP | PBE0 |
| PBE[U] | -0.39 | -0.21 | -0.22 | -0.23 | -0.22 |
| PBE | -0.08 | 0.06 | 0.06 | 0.04 | 0.07 |
| TPSSh | -0.32 | -0.20 | -0.20 | -0.21 | -0.19 |
| B3LYP | -0.62 | -0.61 | -0.59 | -0.57 | -0.58 |
| PBE0 | -0.94 | -0.84 | -0.83 | -0.84 | -0.83 |
| TPSS | 0.05 | 0.19 | 0.19 | 0.16 | 0.19 |
| TPSS0 | -0.81 | -0.72 | -0.71 | -0.72 | -0.71 |
| M06 | -1.04 | -0.97 | -0.89 | -0.95 | -0.96 |
| M06-L | -0.51 | -0.49 | -0.44 | -0.46 | -0.47 |
| M06L-2X | -1.52 | -1.63 | -1.62 | -1.51 | -1.59 |
| PBE[HF] | -1.31 | -1.26 | -1.24 | -1.25 | -1.24 |

Table S5: $\Delta E_{\text{H-L}}$ (eV) of $Fe(CO)_6]^{2+}$ computed with different functionals using five geometries (PBE+U, PBE, TPSSh, B3LYP, PBE0).

| | $\Delta E_{\text{H-L}}$ | | | | |
|---|---|---|---|---|---|
| Geometry → Functional ↓ | PBE+U | PBE | TPSSh | B3LYP | PBE0 |
| PBE[U] | 2.41 | 3.19 | 3.07 | 2.94 | 3.10 |
| PBE | 3.06 | 3.45 | 3.63 | 3.39 | 3.44 |
| TPSSh | 2.01 | 2.23 | 2.25 | 2.23 | 2.24 |
| B3LYP | 1.16 | 1.23 | 1.25 | 1.27 | 1.24 |
| PBE0 | 1.10 | 1.34 | 1.34 | 1.32 | 1.35 |
| TPSS | 2.79 | 3.05 | 3.07 | 3.04 | 3.06 |
| TPSS0 | 0.97 | 1.07 | 1.10 | 1.11 | 1.10 |
| M06 | 0.88 | 0.91 | 1.03 | 0.99 | 0.97 |
| M06-L | 1.68 | 1.78 | 1.78 | 1.83 | 1.81 |
| M06L-2X | -1.10 | -1.64 | -1.54 | -1.37 | -1.55 |
| PBE[HF] | 0.27 | 0.66 | 0.58 | 0.52 | 0.60 |

Table S6: Metal-ligand bond distances (in Å).

| Complex | Spin state | PBE+U | PBE | TPSSh | B3LYP | PBE0 |
|---|---|---|---|---|---|---|
| $[Fe(NH_3)_6]^{2+}$ | LS | 2.16 | 2.07 | 2.08 | 2.11 | 2.08 |
| | HS | 2.32 | 2.29 | 2.28 | 2.31 | 2.28 |
| $[Fe(CO)_6]^{2+}$ | LS | 2.02 | 1.90 | 1.93 | 1.95 | 1.92 |
| | HS | 2.36 | 2.25 | 2.30 | 2.32 | 2.29 |

Table S7: $U_{\text{sc}}$ computed at each geometry.

| Complex | Spin state | PBE+U | PBE | TPSSh | B3LYP | PBE0 |
|---|---|---|---|---|---|---|
| $[Fe(NH_3)_6]^{2+}$ | LS | 7.37 | 7.30 | 7.29 | 7.30 | 7.29 |
| | HS | 6.33 | 6.24 | 6.23 | 6.26 | 6.23 |
| $[Fe(CO)_6]^{2+}$ | LS | 9.22 | 10.13 | 9.89 | 9.69 | 9.96 |
| | HS | 6.51 | 6.74 | 6.61 | 6.55 | 6.62 |

Table S8: Lattice parameters computed using PBE+D3+BJ (see text) for the molecular crystals.

| Complex | | a | b | c | $\alpha$ | $\beta$ | $\gamma$ |
|---|---|---|---|---|---|---|---|
| $Fe(phen)_2(NCS)_2$ | LS | 12.73 | 10.14 | 17.09 | 90.00 | 90.00 | 90.00 |
| | HS | 13.14 | 10.02 | 17.14 | 90.00 | 90.00 | 90.00 |
| $Fe(abpt)_2(NCS)_2$ | LS | 8.52 | 10.05 | 15.96 | 89.66 | 91.86 | 89.72 |
| | HS | 8.60 | 10.41 | 15.81 | 89.81 | 91.12 | 89.76 |
| $Fe(abpt)_2(NCSe)_2$ | LS | 8.59 | 10.06 | 16.06 | 89.71 | 91.17 | 89.76 |
| | HS | 8.66 | 10.37 | 15.90 | 89.86 | 90.50 | 89.80 |
| $Fe[HB(pz)_3]_2$ | LS | 9.84 | 17.23 | 12.78 | 90.73 | 95.75 | 91.10 |
| | HS | 9.71 | 17.57 | 13.17 | 89.94 | 97.31 | 90.06 |
| $FeL_2[BF_4]_2$ | LS | 8.61 | 8.64 | 18.33 | 89.98 | 95.39 | 90.00 |
| | HS | 8.55 | 8.61 | 18.63 | 90.00 | 94.93 | 90.00 |

## $\Delta\rho$ analysis

We extract the PBE, PBE+$U_{sc}$ and PBE+$U_{sc}$+$V_{sc}$ all-electron charge density using Quantum ESPRESSO *pp.x* utility program. The generated Gaussian cube files contain voxel volume elements with side length of 0.103925 Bohr. The same exact voxel volumes are used in the HF and CASPT2 cube files generated using Multiwfn[S20] from the files in Molden format written by ORCA and BAGEL,[S21] respectively. We employ the Bader charge analysis code by Henkelman et al.[S22–S25] to extract the Fe electron charge density $\rho^{Fe}(r)$.

## References


(S1) Mariano, L. A.; Vlaisavljevich, B.; Poloni, R. *J. Chem. Theory Comput.* **2020**, *16*, 6755–6762.

(S2) Giannozzi, P.; Baroni, S.; Bonini, N.; Calandra, M.; Car, R.; Cavazzoni, C.; Ceresoli, D.; Chiarotti, G. L.; Cococcioni, M.; Dabo, I.; Corso, A. D.; Fabris, S.; Fratesi, G.; de Gironcoli, S.; Gebauer, R.; Gerstmann, U.; Gougoussis, C.; Kokalj, A.; Lazzeri, M.; Martin-Samos, L.; Marzari, N.; Mauri, F.; Mazzarello, R.; Paolini, S.; Pasquarello, A.; Paulatto, L.; Sbraccia, C.; Scandolo, S.; G. Sclauzero, A. P. S.; Smogunov, A.; Umari, P.; Wentzcovitch, R. M. *J. Phys: Condens. Matter* **2009**, *21*, 395502.

(S3) Giannozzi, P.; Andreussi, O.; Brumme, T.; Bunau, O.; Nardelli, M. B.; Calandra, M.; Car, R.; Cavazzoni, C.; Ceresoli, D.; Cococcioni, M.; Colonna, N.; Carnimeo, I.; Corso, A. D.; de Gironcoli, S.; Delugas, P.; Jr, R. A. D.; Ferretti, A.; Floris, A.; Fratesi, G.; Fugallo, G.; Gebauer, R.; Gerstmann, U.; Giustino, F.; Gorni, T.; Jia, J.; Kawamura, M.; Ko, H.-Y.; Kokalj, A.; KÃijÃğÃijkbenli, E.; Lazzeri, M.; Marsili, M.; Marzari, N.; Mauri, F.; Nguyen, N. L.; Nguyen, H.-V.; de-la Roza, A. O.; Paulatto, L.; PoncÃľ, S.; Rocca, D.; Sabatini, R.; Santra, B.; Schlipf, M.; Seitsonen, A. P.; Smo-

gunov, A.; Timrov, I.; Thonhauser, T.; Umari, P.; Vast, N.; Wu, X.; Baroni, S. *Journal of Physics: Condensed Matter* **2017**, *29*, 465901.

(S4) Garrity, K. F.; Bennett, J. W.; Rabe, K. M.; Vanderbilt, D. *Comp. Mater. Sci.* **2014**, *81*, 446–452.

(S5) Bennett, J. W.; Hudson, B. G.; Metz, I. K.; Liang, D.; Spurgeon, S.; Cui, Q.; Mason, S. E. *Comp. Mater. Sci.* **2019**, *170*, 109137.

(S6) Makov, G.; Payne, M. C. *Phys. Rev. B* **1995**, *51*, 4014–4022.

(S7) Neese, F. *WIREs Comput. Mol. Sci.* **2012**, *2*, 73–78.

(S8) Blöchl, P. E. *Phys. Rev. B* **1994**, *50*, 17953–17979.

(S9) Corso, A. D. *Comp. Mater. Sci.* **2014**, *95*, 337–350.

(S10) Grimme, S.; Antony, J.; Ehrlich, S.; Krieg, H. *J. Chem. Phys.* **2010**, *132*, 154104.

(S11) Smith, D. G. A.; Burns, L. A.; Patkowski, K.; Sherrill, C. D. *J. Phys. Chem. Lett.* **2016**, *7*, 2197–2203.

(S12) Phung, Q. M.; Feldt, M.; Harvey, J. N.; Pierloot, K. *J. Chem. Theory Comput.* **2018**, *14*, 2446–2455.

(S13) Feller, D. *The Journal of Chemical Physics* **1992**, *96*, 6104–6114.

(S14) Feller, D. *The Journal of Chemical Physics* **1993**, *98*, 7059–7071.

(S15) Helgaker, T.; Klopper, W.; Koch, H.; Noga, J. *The Journal of Chemical Physics* **1997**, *106*, 9639–9646.

(S16) Cococcioni, M.; De Gironcoli, S. *Phys. Rev. B* **2005**, *71*, 035105.

(S17) Campo Jr, V. L.; Cococcioni, M. *J. Phys.-Condens. Mat.* **2010**, *22*, 055602.

(S18) Timrov, I.; Marzari, N.; Cococcioni, M. *Phys. Rev. B* **2018**, *98*, 085127.

(S19) Kulik, H. J.; Cococcioni, M.; Scherlis, D. A.; Marzari, N. *Phys. Rev. Lett.* **2006**, *97*, 103001.

(S20) Lu, T.; Chen, F. *J. Comput. Chem.* **2012**, *33*, 580–592.

(S21) Shiozaki, T. *WIREs Comput. Mol. Sci* **2018**, *8:e1331*.

(S22) Henkelman, G.; Arnaldsson, A.; Jónsson, H. *Computational Materials Science* **2006**, *36*, 354–360.

(S23) Sanville, E.; Kenny, S. D.; Smith, R.; Henkelman, G. *Journal of Computational Chemistry* **2007**, *28*, 899–908.

(S24) Tang, W.; Sanville, E.; Henkelman, G. *Journal of Physics: Condensed Matter* **2009**, *21*, 084204.

(S25) Yu, M.; Trinkle, D. R. *J. Chem. Phys.* **2011**, *134*, 064111.
